# Supplementary material for: Escaping kinetic traps using non-reciprocal interactions
Source: arXiv:2309.00562 ancillary file (2024-07-12)
Supplement: Supplementary file 1 [file SM_EscKinTra.pdf]

# Escaping kinetic traps using non-reciprocal interactions

## *Supplemental Material*

Saeed Osat,<sup>1,\*</sup> Jakob Metson,<sup>1,†</sup> Mehran Kardar,<sup>2</sup> and Ramin Golestanian<sup>1,3,‡</sup>

<sup>1</sup>*Max Planck Institute for Dynamics and Self-Organization (MPI-DS), 37077 Göttingen, Germany*

<sup>2</sup>*Department of Physics, Massachusetts Institute of Technology, Cambridge, MA 02139, United States*

<sup>3</sup>*Rudolf Peierls Centre for Theoretical Physics, University of Oxford, Oxford OX1 3PU, United Kingdom*

(Dated: July 12, 2024)

## CONTENTS

|                                                  |   |
|--------------------------------------------------|---|
| I. Non-Reciprocal Multifarious Self-Organization | 2 |
| A. Reciprocal interactions                       | 2 |
| B. Non-reciprocal interactions                   | 2 |
| II. Monte-Carlo simulation                       | 2 |
| III. Error calculation                           | 3 |
| IV. Coloring                                     | 3 |
| V. Interface detection                           | 3 |
| A. Suppressing nucleation                        | 4 |
| B. Interface displacement                        | 4 |
| C. Time scales                                   | 5 |
| VI. Defect nucleation                            | 5 |
| VII. Supplemental Video Descriptions             | 5 |
| References                                       | 6 |

---

\* These authors contributed equally to this work; [saeed.osat@ds.mpg.de](mailto:saeed.osat@ds.mpg.de)

† These authors contributed equally to this work

‡ [ramin.golestanian@ds.mpg.de](mailto:ramin.golestanian@ds.mpg.de)

## I. NON-RECIPROCAL MULTIFARIOUS SELF-ORGANIZATION

We consider  $m$  target structures which are random permutations of  $M$  tiles.  $q$  of the target structures are arranged in a sequence  $S^1 \rightarrow S^2 \rightarrow \dots \rightarrow S^{q-1} \rightarrow S^q$ . The goal is to design interactions with a reciprocal part that guarantees the correct retrieval of each of the structures and a non-reciprocal part that provides the shifting between these structures in a predefined order.

### A. Reciprocal interactions

First, we define  $\mathcal{I}^r$  as the set of all specific interactions imposed by all  $m$  structures. This set is a union of smaller sets that each contain the specific interactions imposed by one of the target structures,  $\mathcal{I}^r \equiv I^r(S^1) \cup I^r(S^2) \cup \dots \cup I^r(S^m)$ . Each of these smaller sets can be explicitly defined as

$$I^r(S^\ell) = \bigcup_{\langle \alpha, \beta \rangle} S_\alpha^\ell \square S_\beta^\ell, \quad (\text{S1})$$

where  $\alpha$  and  $\beta$  are lattice coordinates  $(i, j)$  running over nearest neighbors. To enable clear notation we rotate the lattice as shown in Figure S1(a).  $\square \in \{\searrow, \swarrow\}$  is the direction of the specific interaction, horizontal or vertical as shown in Figure S1(b). The interaction matrix in units of the thermal energy  $k_B T$  is

$$U_{A\square B}^r = \begin{cases} -\varepsilon, & \text{if } A\square B \in \mathcal{I}^r, \\ 0, & \text{otherwise.} \end{cases} \quad (\text{S2})$$

The configuration of a system at any time can be captured by the configuration variable  $\sigma_\alpha$ .  $\sigma_\alpha = 1, 2, \dots, M$  represents different tile species, while  $\sigma_\alpha = 0$  stands for an empty grid point. A (classical generalized) Hamiltonian for the system using this configuration variable and interaction potential  $U$  is defined as:

$$\mathcal{H} = \sum_{\langle \alpha, \beta \rangle} U_{\sigma_\alpha \square \sigma_\beta}^r - \mu n, \quad (\text{S3})$$

where  $\mu$  is the chemical potential of the tiles. In our case we assume  $\mu$  is the same for all tiles.  $n = \sum_\alpha (1 - \delta_{0, \sigma_\alpha})$  counts the total number of tiles (non-empty grid points) in a given configuration, and  $\square \in \{\searrow, \swarrow\}$ . Note that the chemical potential is related to the average density of tiles in the system.

### B. Non-reciprocal interactions

To begin, consider a single shift  $S^\ell \rightarrow S^{\ell+1}$ . A tile will approach and interact with the neighbors of its counterpart in the previous pattern in the sequence. The set of all non-reciprocal interactions imposed for this shift is

$$I^{\text{nr}}(S^{(\ell)} \rightarrow S^{(\ell+1)}) = \bigcup_{i,j} \left\{ S_{i-1,j}^{(\ell)} \swarrow S_{i,j}^{(\ell+1)}, S_{i,j}^{(\ell+1)} \nearrow S_{i+1,j}^{(\ell)}, S_{i,j}^{(\ell+1)} \searrow S_{i,j-1}^{(\ell)}, S_{i,j+1}^{(\ell)} \swarrow S_{i,j}^{(\ell+1)} \right\}. \quad (\text{S4})$$

The set of all non-reciprocal interactions for the full sequence is denoted  $\mathcal{I}^{\text{nr}} \equiv I^{\text{nr}}(S^1 \rightarrow S^2) \cup \dots \cup I^{\text{nr}}(S^{q-1} \rightarrow S^q)$ . We define

$$R_{A \blacksquare B}^{\text{nr}} = \begin{cases} \lambda, & \text{if } A \blacksquare B \in \mathcal{I}^{\text{nr}}, \\ 0, & \text{otherwise,} \end{cases} \quad (\text{S5})$$

where  $\blacksquare \in \{\swarrow, \nwarrow, \nearrow, \searrow\}$  represents all possible specific non-reciprocal interactions, respecting direction, as shown in Figures S1(c) and (d).

## II. MONTE-CARLO SIMULATION

Either the system is defined as a square lattice of size  $2\sqrt{M} \times 2\sqrt{M}$ , in which  $\sqrt{M} \times \sqrt{M}$ -sized target structures are embedded, or the system size is the same as the pattern size with  $L_x \times L_y = M$ . This can be rectangular, or

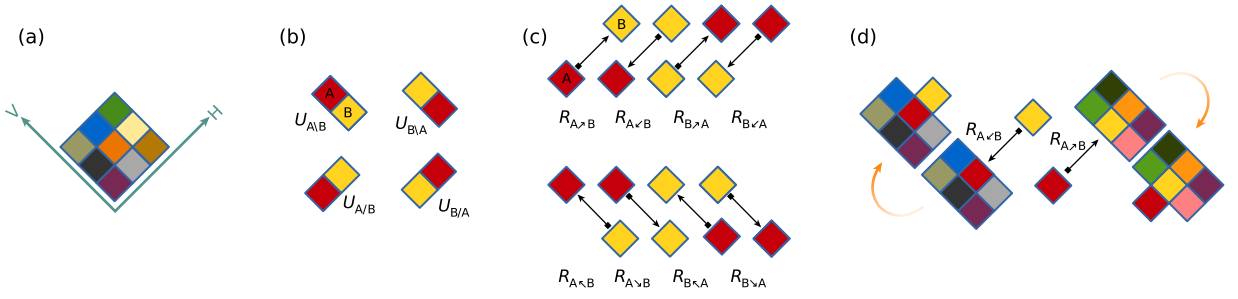

FIG. S1. Directionality of interactions. (a) Lattice rotated  $45^\circ$  anticlockwise to enable clear notation of interaction direction. (b) Reciprocal and (c) non-reciprocal interaction directions. (d)  $B$  arriving next to  $A$  is different to  $A$  arriving next to  $B$ .

square with  $L_x = L_y = L$ . We employ a condition of full heterogeneity and zero sparsity, meaning each structure represents a random permutation of the different tile species. To simulate this system, we utilize a generalized version of the grand canonical Monte Carlo method. In each Monte Carlo step, a random lattice point  $(i, j)$  is selected, and its component  $\sigma_{i,j}$  is replaced by another random component  $\sigma'$  with probability

$$p = \min\{1, \exp(\Lambda - \Delta\mathcal{H})\}, \quad (\text{S6})$$

where

$$\Lambda_{i,j} = R_{\sigma_{i-1,j} \searrow \sigma'}^{\text{nr}} + R_{\sigma' \nearrow \sigma_{i+1,j}}^{\text{nr}} + R_{\sigma' \searrow \sigma_{i,j-1}}^{\text{nr}} + R_{\sigma_{i,j+1} \nwarrow \sigma'}^{\text{nr}}. \quad (\text{S7})$$

The  $\lambda \rightarrow 0$  limit of this model corresponds to the equilibrium MSA model.

### III. ERROR CALCULATION

We use two different algorithms to calculate the error of the self-assembly:

1) *System size equals pattern size.* Since the pattern and system size are the same, a direct comparison of each grid point in the system and the pattern  $S^i$  gives the overlap  $O_i$ . Error is defined as  $e_i = 1 - O_i$ .

2) *Pattern is embedded in the system.* (a) find the largest connected cluster of the tiles  $L$ , (b) construct  $A = L \cup S^i$ , the union of the desired structure as located at the center of the lattice  $S^i$  and  $L$ , and (c) calculate  $O_i = |A \cap S^i|/|A|$ . The error is  $e_i = 1 - O_i$ , which is defined for each single desired structure.

Note that with shape-shifting one needs to get the minimum error over all patterns in the shifting sequence.

### IV. COLORING

Since a pattern is made of  $M$  distinct tiles, a configuration of the system is hard to visually interpret. In this regard, we show the configuration of the system in terms of assembled patterns. The first step is to assign a unique color to each of the patterns. The appearance of one of these colors in the system means that part of the system is assembled or filled with the pattern corresponding to that color. Empty lattice points are colored white. There are again the two cases:

1) *System size equals pattern size.* Each tile in the system inherits the color of a pattern that shares the same lattice point. In the uncommon event of a tie, we pick randomly from the tied colors.

2) *Pattern is embedded in the system.* Tiles are colored based on specific interactions with their neighbors. When a tile does not have any specific interactions with its neighbors, a random color is assigned from the set of  $m$  unique colors. Otherwise, a tile inherits the color of the pattern that contributes the most to the specific interactions of this tile with its neighbors. In the case of a tie, the tile selects a color randomly from the set of competing patterns.

### V. INTERFACE DETECTION

We have developed an algorithm that effectively detects the interface, as illustrated in Fig. S2. The simulation begins with an initial configuration where a slab of structure  $S^2$  serves as the substrate. The top interface of this

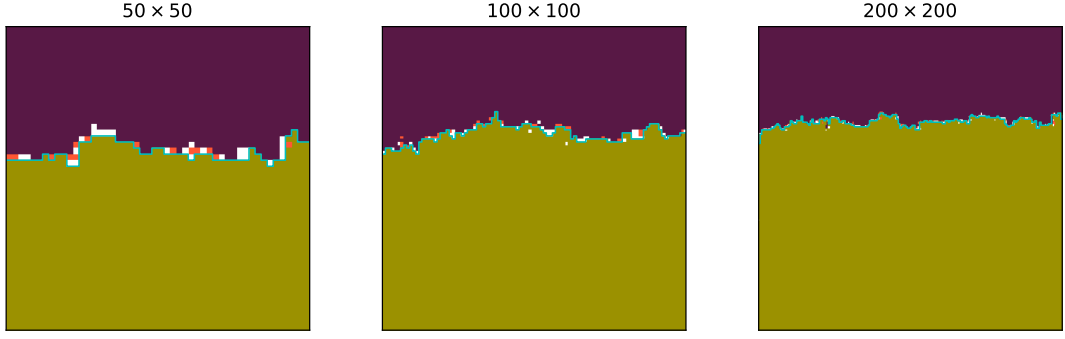

FIG. S2. Detection of interface. The algorithm defined in the text can robustly detect the growing interface. Dark blue region correspond to pattern  $S^1$ . Green region corresponds to growing pattern  $S^2$ . White areas show empty lattice points. Red regions show those grid points that host a wrong tile that does not correspond to neither of target patterns. See Supplemental Video 1 for evolution of the interface. The simulation parameters are  $(\varepsilon, \mu, \lambda) = (11, -20, 7.3)$

substrate starts to evolve and grow. To obtain the interface, we identify all lattice points that contain tiles matching pattern  $S^2$ . These tiles form distinct clusters within the system. At this stage, we assume that the initial substrate corresponds to the largest cluster, and its height represents the interface, as depicted in Fig. S2. It is important to note that this assumption holds true only if we prevent the nucleation of pattern  $S^2$  in other regions of pattern  $S^1$  that have not undergone shifting.

### A. Suppressing nucleation

For sufficiently strong  $\lambda$ , shifts occur in the system. These shifts begin with the nucleation of a small seed within the current structure. The interface of the new phase (structure) droplet can grow and merge with the existing interface. This sudden jump in interface height can significantly affect the overall statistics of the interface. To address this issue, we introduced a criterion based on the minimum and maximum height of the current interface. Only updates with  $y$ -coordinates within the range  $[h_{\min} - 5, h_{\max} + 5]$  are accepted, while any updates outside this range are discarded. This condition effectively suppresses the nucleation of new droplets and helps maintain the integrity of the interface. However, it should be noted that as the system size increases, the domain  $[h_{\min} - 5, h_{\max} + 5]$  also expands, increasing the probability of nucleation in this region.

### B. Interface displacement

The system under consideration is a 2D square or rectangular lattice. Previous study have demonstrated that non-reciprocal interactions lead to shifts that occur on a different timescale than to the retrieval time of structures. As a result, the interface starts from a small  $y$  value in the substrate and rapidly reaches the top of the structure. This hinders the ability of the interface to undergo roughening and reach saturation. To address this issue, two possible solutions have been proposed:

One solution is to consider a thin rectangular system. For example, in Supplemental Video 2, a  $40 \times 400$  rectangular system is shown. The elongated shape of the system allows the small interface to undergo roughening and reach saturation. However, this approach suffers from long simulation times due to the scaling of interface growth with the system size. At each lattice sweep ( $L_x \times L_y$ ), a point on the interface has a chance to update itself. However, an update occurs with a high probability only if the correct tile among all the tiles has been selected, which happens every  $(L_x \times L_y)$  lattice sweep. Therefore, the inherent timescale of interface growth scales with the number of the distinct tiles (in our case area of the pattern), making a long rectangular system unsuitable for simulating long interfaces.

The second approach is to use interface displacement or two-phase method. In this method, starting from a  $L_x \times L_y$  lattice, whenever the interface reaches or gets close to  $L_y$ , we move it down to smaller values of  $y$ . It is important to note that we do not change the geometry of the interface during this displacement. Then, we initialize the lattice with all points below the interface as structure two and all points above the interface as structure one. However, it is worth mentioning that the stochastic noise below the interface is lost in this method.

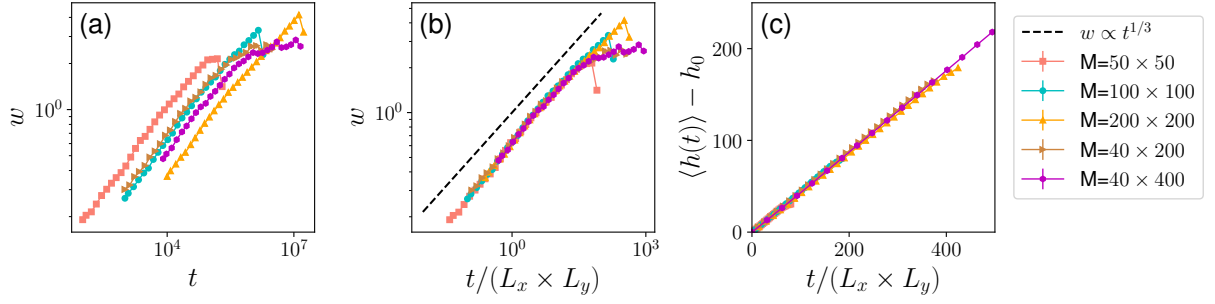

FIG. S3. System size and time scale. (a) shows roughness for different lattice sizes. Saturation happens for thin rectangular systems, such as  $40 \times 400$ .  $t$  is the number of lattice sweep Monte-Carlo steps. Note that a point on the interface not only waits on average one lattice sweep to have the chance of update but also waits on average  $M$  steps (corresponding to the total number of tiles in the system) in order to pick up the right tile.  $M = L_x \times L_y$  for 2D lattices. Rescaling the time scales in all the plots with  $M$  causes the curves to overlap as shown in (b). Note that these plots lack saturation due to finite system size. (c) shows the velocity of the interface in all cases for a fixed values of  $(\varepsilon, \mu, \lambda) = (11, -20, 7.3)$ .

By comparing the simulation results of long rectangular systems with those of smaller systems using interface displacement, we can confirm that the statistics of the interface in both cases match, as illustrated in Fig. S3 (b) and (c).

### C. Time scales

Consider a rectangular system of size  $L_x \times L_y$ , with the same size as the patterns, which consist of  $M = L_x \times L_y$  tiles. On average, each lattice sweep (consisting of  $L_x \times L_y$  moves) allows each lattice point to attempt an update by replacing its current tile with a randomly selected tile. Since the tile selection is random, the probability of selecting the correct tile in the shifting sequence is  $1/(L_x \times L_y)$ . In other words, for a lattice point, it takes  $L_x \times L_y$  lattice sweeps to select the correct tile.

Let us compare this with simple (1+1)-D interface growth. In this case, a sweep gives each point on the interface an opportunity to update its height. In 2D, a lattice sweep is equivalent to sweeping the 1D interface. However, due to the tile selection criteria, it now takes  $L_x \times L_y$  sweeps for the interface to update its height. Therefore, in order to compare systems of different sizes, we need to rescale time  $t$  (measured in lattice sweeps) by the number of distinct tiles, which is  $L_x \times L_y$ . Figure S3 demonstrates the necessity of rescaling time to accurately capture the timing of the interface evolution in systems of various sizes.

## VI. DEFECT NUCLEATION

To measure the nucleation time of two  $S^2$  inside  $S^1$  with a non-reciprocal sequence  $S^1 \rightarrow S^2$ , we fill the system completely with  $S^1$  and then measure how long it takes for 25% of the system to be filled with  $S^2$ . We choose 25% as it is sufficiently large to avoid counting small unsuccessful nucleations and fluctuations as successful nucleation events. Supplemental Video 4 shows an example of  $S^2$  nucleating inside  $S^1$ . To apply this to escaping from kinetic traps, consider a system trapped in a chimera formed from a slab of  $S^1$  and a slab of  $S^3$ , with shifting sequence  $S^1 \rightarrow S^2 \rightarrow S^3$ . With this sequence there is no direct route for the interface to grow and order for the system to escape this kinetic trap, first  $S^2$  needs to nucleate inside the  $S^1$  region. Once the nucleated  $S^2$  region reaches the  $S^1 - S^3$  interface a defect is formed where the three regions meet, which proceeds to lead the system out of the trap to end in a fully assembled  $S^3$  two. Therefore, the nucleation time is a quantity of interest for defect-mediated escape.

## VII. SUPPLEMENTAL VIDEO DESCRIPTIONS

### • Supplemental Video 1

Interface fluctuations depend on  $\lambda$ . A system of size  $50 \times 50$  has been used for simulation and  $(\varepsilon, \mu) = (24, -38)$ .  $\lambda = 16$  and  $\lambda = 24$  shown in red are the closest values to  $\lambda_{min} = \frac{2}{3}\varepsilon$  and  $\lambda_{max} = \varepsilon$ .

- **Supplemental Video 2**

A  $40 \times 400$  rectangular system is shown. The elongated shape of the system allows the small interface to undergo roughening and reach saturation. However, this approach suffers from long simulation times due to the scaling of interface growth with the system size.

- **Supplemental Video 3**

The algorithm defined in the main text can robustly detect the growing interface. The simulation parameters are  $(\varepsilon, \mu, \lambda) = (11, -20, 7.3)$ .

- **Supplemental Video 4**

Nucleation of pattern  $S^2$  within  $S^1$ , with sequence  $S^1 \rightarrow S^2$ .

$$\sqrt{M} = 50, L = 50$$

4 patterns; sequence  $S^1 \rightarrow S^2$

$$(\varepsilon, \mu, \lambda) = (24, -38, 20)$$

- **Supplemental Video 5**

A small droplet of  $S^2$  placed on the  $S^1$ - $S^3$  boundary is destroyed by the chasing  $S^3$  pattern. This leaves the system trapped in a chimeric state.

$$\sqrt{M} = 50, L = 50, \text{ initial droplet radius} = 6$$

4 patterns; sequence  $S^1 \rightarrow S^2 \rightarrow S^3 \rightarrow S^4 \rightarrow S^1$

$$(\varepsilon, \mu, \lambda) = (24, -38, 16)$$

- **Supplemental Video 6**

A large droplet of  $S^2$  placed on the  $S^1$ - $S^3$  boundary allows the system to escape the chimeric state, leaving the system in a fully assembled  $S^3$  state.

$$\sqrt{M} = 50, L = 50, \text{ initial droplet radius} = 11$$

4 patterns; sequence  $S^1 \rightarrow S^2 \rightarrow S^3 \rightarrow S^4 \rightarrow S^1$

$$(\varepsilon, \mu, \lambda) = (24, -38, 16)$$


---
